# Supplementary material for: Ultrafast pulse measurement via time-domain single-pixel imaging
Source: arXiv:2009.13693 source file (2021-04-23)
Supplement: Supplementary file 1 [file Supplement_compressive_ultrafast_sensing_enabled_by_programmable_temporal_fan_out.pdf]

# Supplementary Information of compressive ultrafast sensing enabled by programmable temporal fan-out

Jiapeng Zhao,<sup>1, a)</sup> Jianming Dai,<sup>2</sup> Boris Braverman,<sup>3</sup> Xi-Cheng Zhang,<sup>1</sup> and Robert W. Boyd<sup>1, 3</sup>

<sup>1)</sup>*The Institute of Optics, University of Rochester, Rochester, New York, 14627, USA*

<sup>2)</sup>*Center for Terahertz Waves and School of Precision Instruments & Opto-Electronics Engineering, Tianjin University, Tianjin, 300072, PR China*

<sup>3)</sup>*Department of Physics, University of Ottawa, Ottawa, K1N 6N5, Canada*

---

<sup>a)</sup>Electronic mail: jzhao24@ur.rochester.edu

## I. THEORETICAL MODEL AND COMPRESSIVE SENSING

We first assume that our input ultrafast pulse is horizontally polarized, and has a carrier frequency of  $\omega_0$  with a pulse duration equal to  $\tau_w$ . We can write the input pulse  $E_{in}(x, y, z, \omega_0, t)$  propagating in the  $z$  direction as the following:

$$E_{in}(x, y, z, \omega_0, t) = A_0(x, y) \exp\left(-\frac{t^2}{\tau_w^2}\right) \exp(i\omega_0 t + i\vec{k} \cdot \vec{z}), \quad (1)$$

where  $A_0(x, y)$  is the transverse amplitude distribution. Since the input pulse is propagating along  $z$  direction, the dot product of wave vector  $\vec{k}$  and longitudinal coordinate  $\vec{z}$  will be just a scalar product  $kz$ . After TFO gate, we get a sequence of replicas  $E_{TFO}(x, y, z, \omega_0, t)$  which are separated by the temporal interval  $\Delta\tau$ :

$$E_{TFO}(x, y, z, \omega_0, t) = \sum_j A_j(x, y) \exp\left(-\frac{(t - j\Delta\tau)^2}{\tau_w^2}\right) \exp(i\omega_0(t - j\Delta\tau) + i\vec{k}_j \cdot \vec{z}), \quad (2)$$

where  $A_j(x, y)$  is the amplitude of the  $j$ th replica and can be individually modulated by turning on different amounts of mirrors in each column of DMD. Due to the spread in the direction of wave vectors, each replica will have a different wave vector  $\vec{k}_j$ . Then the dot product of  $\vec{k}_j$  and  $\vec{z}$  can be written as  $k_j z \cos \theta_j$ , where  $\theta_j$  is the angle between two vectors. However, since the maximal  $\theta_j$  in our case is only 0.01 rad,  $k_j z \cos \theta_j$  can be approximated as  $kz$  so that we will get the following final form of TFO outputs  $E_{TFO}(x, y, z, \omega_0, t)$ :

$$E_{TFO}(x, y, z, \omega_0, t) = \sum_j A_j(x, y) \exp\left(-\frac{(t - j\Delta\tau)^2}{\tau_w^2}\right) \exp(i\omega_0(t - j\Delta\tau) + ikz), \quad (3)$$

which represents a sequence of pulses with duration  $\tau_w$  and amplitude  $A_j(x, y)$  located at temporal position  $j\Delta\tau$ . Therefore, we successfully build a TFO gate using a DMD and a lens L1 within the Rayleigh range of the focus. One can further remove the spatial dependence by coupling these TFO replicas into a single mode fiber. Hence then, at the focus of L1, we get programmable pulse trains containing temporal replicas of the original input ultrafast pulse, and each replica has its individual temporal position and amplitude under deterministic control. Meanwhile, a much larger  $T$  is available if one uses the output of a frequency comb as the input source of our TFO gate.

Our THz measurement is based on the free-space electro-optic (EO) effect<sup>1-3</sup>. THz pulses introduce birefringence in EO crystals which change the polarization of the probe beam. By using the quarter wave plate (QWP) and Wollaston prism, the probe beam will be separated

into two orthogonal polarizations with equal intensity. If THz pulses do not interact with probe pulses, balanced detectors will yield no response. Otherwise, polarization state of probe pulses will be modified leading to the unequal intensities of two polarizations, which further results in a signal  $P_s$  on balanced detectors:

$$P_s = \int \int \frac{1}{c} |E_{\text{TFO}}(x, y, \omega_0, t)|^2 \omega_0 L n_0^3(\omega_0) r_{41} E_{\text{THz}}(x, y, \omega_{\text{THz}}, t) dx dy dt, \quad (4)$$

where  $c$  is the speed of light in vacuum.  $L$  is the thickness of the detection crystal, and  $\omega_0$  is the frequency of probe.  $n_0(\omega_0)$  is the refractive index of the detection crystal at frequency  $\omega_0$ , and  $r_{41}$  is the EO efficient of the detection crystal. From Eqn. (4), we can see that the THz pulse can only be detected when that part of the THz pulse is temporally coinciding with a TFO replica. Therefore, temporally modulating the structure of TFO output  $E_{\text{TFO}}(x, y, z, \omega_0, t)$  is equivalent to temporally modulating the THz field in the same manner but leaving the probe field unchanged. However, temporally encoding the probe beam using our ultrafast TFO gate can simply use commercially available NIR DMDs, and further release the requirement of ultrafast THz temporal modulator, which, to the best of our knowledge, has not been reported yet.

Now we assume that our THz pulse is temporally sampled  $N$  times, and the measured pulse can be represented by a  $N$  dimensional vector  $\psi$ . The measurement basis is  $S$  and the corresponding coefficient vector is  $\phi$ . The basic idea of compressive sensing comes from the fact that, for a  $N$  dimensional vector  $\psi$ , it is possible to find a basis  $R$  that most coefficients in the coefficient vector  $\phi$  are zero or very small. What the CS does is to exploit the sparsity of the signal vector, through optimization, to recover most information by only adopting those nonzero coefficients. Therefore, one can beat the Nyquist sampling limit by sub-sampling the signal without losing too much information. To successfully implement CS, two conditions have to be fulfilled: the sparsity of the signals of interest, and the incoherence of sensing basis  $S$  and recovery basis  $R^4$ .

Sparsity pertains to the signals of interest that is independent of the choice of sensing basis. Luckily, most signals in nature are sparse if they are represented in convenient bases<sup>4</sup>. Therefore, in most cases, we don't have to worry about the first condition. The second condition requires that the sampling and recovery bases are mutually incoherent. The coherence between two bases is defined as the largest correlation between any two elements in

$S$  and  $R$ :

$$\mu(S, R) = \sqrt{N} \times \max |\langle S_k, R_j \rangle|, \quad (5)$$

where  $N$  is the dimension of the basis and  $1 \leq k, j \leq N$ . Therefore, two bases are maximally incoherent when  $\mu(S, R) = 1$ . One example of maximally incoherent bases is the Fourier conjugate bases (for example time-frequency). Therefore, sensing the signals in the Fourier domain is a good idea, which leads to the use of Walsh ordered Hadamard matrix in our case. However,  $R$  and  $S$  are not necessarily Fourier conjugate bases of each other, and in the optimization process, CS will explore the optimal recovery basis depending on the sensing basis. Therefore, the improvement in measurement efficiency of our approach is fundamental and independent of the basis choice, which means that the use of Walsh ordered Hadamard matrix is not necessary. Another general choice of the sampling basis is random basis since it has little coherence with any fixed basis ( $\mu(R, S) \sim \sqrt{2 \log N}$ ). This explains why random basis, no matter in spatial ghost imaging or TGI, can always work in CS.

We first assume that the signal  $\psi$  can be measured using basis  $S$  with the measurement result coefficient vector  $\phi$ :  $\phi = S\psi$ . Now we assume that there is a basis  $R$  which is incoherent with  $S$ . If we assume that most coefficients under this representation  $R$  are close or equal to zero, we can recover the signal  $\psi$  by  $\ell_1$ -norm minimization. The solution coefficient vector  $\phi'$  can be found by solving the convex optimization problem<sup>4,5</sup>:

$$\min_{\psi'} \|R\psi'\|_{\ell_1}, \text{ subject to } S\psi' = \phi', \quad (6)$$

where  $\|\cdot\|_{\ell_1}$  is the  $\ell_1$ -norm. If the coherent coefficient between two bases  $Q$  and  $T$  is very little, i.e. two bases are incoherent, the THz field vector  $\psi$  can be reconstructed with  $M \geq O[K \log(N)]$  measurements, where  $K$  is the number of nonzero components of vector  $R\psi$ <sup>6</sup>. Therefore, we can surpass the Nyquist rate but still recover the field with a high fidelity.

From what we describe above, one can see that the goal of using CS is to achieve high fidelity signal recovery via sub-sampling the signal. Therefore, we need to carefully reconsider the use of random basis. Even though random basis is always a choice of sampling basis in spatial or temporal ghost imaging since it is incoherent with any fixed basis, it is not ideal in most cases. Due to the randomness in the sampling process, the recovered signal is usually noisy if one strictly sub-samples the signal. Therefore, when the random basis is used, one usually has to over-sample the signal to average out noise, which loses the point

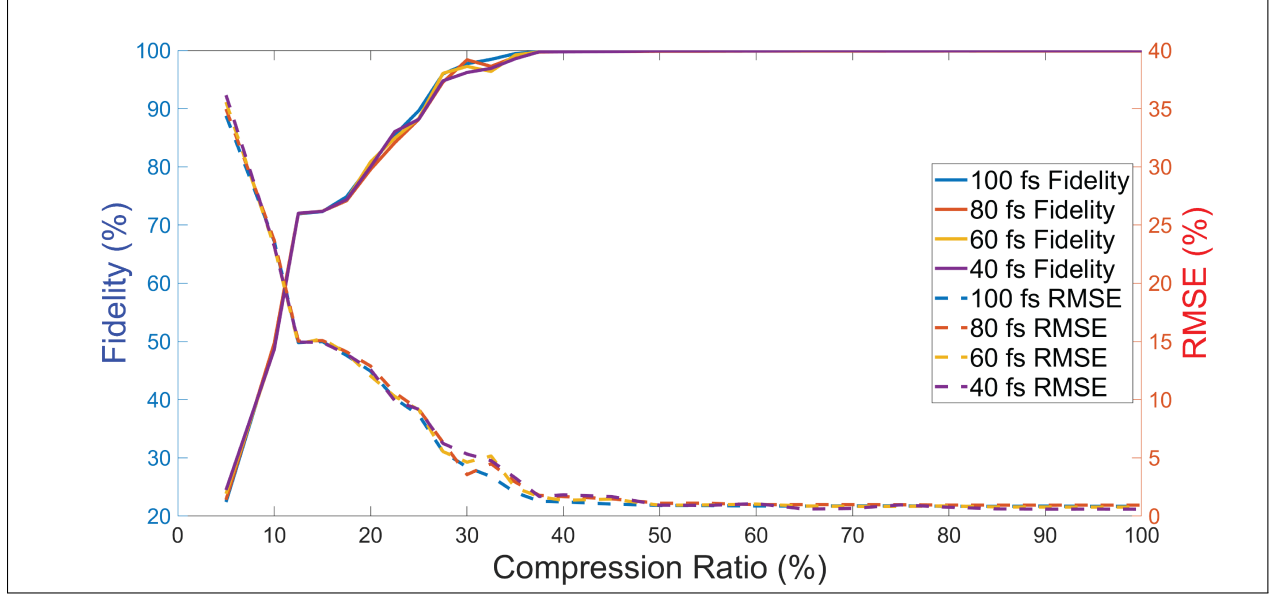

FIG. S1: Fidelity and RMSE of recovered THz pulses as functions of CR under different input pulse durations.

of implementing CS instead. This has been demonstrated in spatial ghost imaging and one can also find the existence of over-sampling in previous TGI systems<sup>7,8</sup>.

From a practical point of view, we use the Total Variation Minimization by Augmented Lagrangian and Alternating Direction Algorithms (TVAL3) package, which provides 4 different total variation based minimization models to solve the minimization problem. The package was provided by Chengbo Li, Wotao Yin and Yin Zhang at Rice University<sup>9</sup>. Fig. S1 shows the simulated fidelity and RMSE as functions of compression ratio (CR) under different pulse durations. We show that the performance of our CTSPI only slightly depends on the pulse duration of the input pulse of TFO gate, which demonstrates that our approach is practical to different pulse durations.

## II. EXAMPLES OF TFO OUTPUTS

Here we would like to show some examples of TFO outputs under different modulations. In Fig. S2(a), the top pulse train has the same envelop as what we use in the experiment (same as the middle one in Fig. 1(c)). After tuning the amount of mirrors in each column of DMD, we can generate a nearly-uniform intensity envelop so that the ratio between the maximum and minimum is only 1.28. Based on this nearly-uniform intensity envelop, we

can further add a temporal structure to it, the same structure shown in the bottom of Fig. 1(c), so that all TFO replicas have similar intensity (Fig. S2(b)). This actually mimics the generation of frequency comb in the temporal domain, and our device is more flexible and can produce more complicated temporal structures. Moreover, as what we show in Fig. S2(c), we can also generate a top-hat pulse with a different pulse duration (3 ps) by turning off different amounts of columns on DMD. Last but not least, we can add a complex intensity envelop as well. For example, in Fig. S2(d), the envelop consists of a V shape envelop with its valley at 6.7 ps and 7 Gaussian distributions centered at 2 ps, 3.7 ps, 5.4 ps, 6.7 ps, 8.4 ps, 9.8 ps and 11.2 ps respectively. Even though the complex structure is not as good as the theoretical design due to the nonuniform illumination of the input pulse, it shows the possibility of arbitrarily engineering the temporal structure of TFO replicas. For all the structures shown above, one can further spend more time to optimize them by tuning the amount of mirrors in each column to compensate the defects from nonuniform illumination. However, this would be beyond the scope of our work.

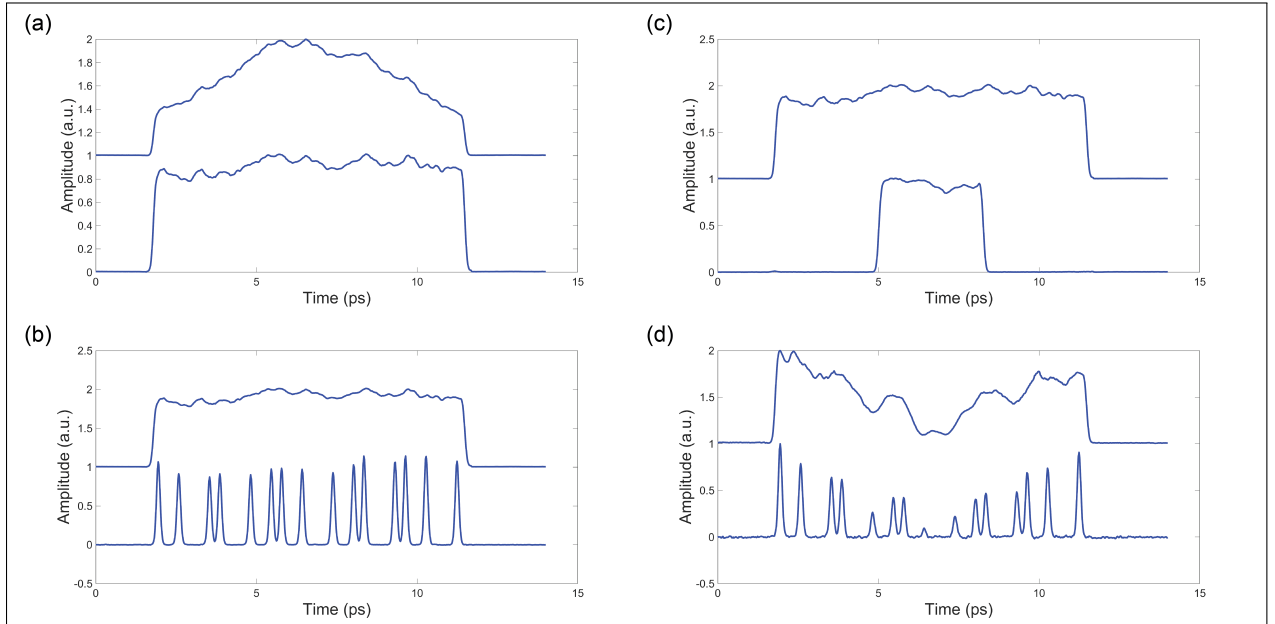

FIG. S2: (a): Modify the envelop closer to a nearly-uniform intensity envelop. (b): Modulate the temporal structure based on a nearly-uniform intensity envelop. (c): Generate a top-hat pulse with 3 ps pulse duration. (d): A complicated intensity envelop and one example of the temporal structure based on it.

### III. MEASURE OPTICAL PULSES USING CTSPI

In optical pulse measurements, we first replace the detection ZnTe crystal with a 1-mm-thick BBO crystal. Then a photomultiplier tube is used as the detector to replace the balanced detector in THz measurements. Next, we combine 5 DMD columns together (80.00 fs) as an effective column. In order to provide enough temporal resolution to resolve optical pulses, we first prepare a set of pulse train and measure the unknown pulse in one time window. Then we shift this window 16.00 fs forward to make another set of measurement, which corresponds to the shift of 1 DMD column. We continue this until 5 shifts are done. The final recovered optical pulse is the average of 5 measurements. Therefore, the temporal resolution in our optical pulse measurement is 16.00 fs. One can further increase the temporal resolution by using a delay stage to shift the time window, which can lead to a temporal resolution less than 5 fs. However, this needs a high-speed synchronization among DMD, delay stage, lock-in amplifier and control computer, which beyond the scope of this paper.

We change the pulse duration in the signal arm by adjusting dispersion induced by the self-phase modulation inside a ZnTe crystal, which is the crystal for THz generation. We move the location of ZnTe crystal to change the intensity of the probe pulse inside it so that the dispersion induced by self-phase modulation is adjusted. The results are shown in Fig. S3. Two optical pulses are measured with different pulse duration ( $\sim 90$  fs and  $\sim 125$  fs). Fig. S3(a) is the compressive measurement result (blue curve) of a 90 fs pulse comparing to the delay stage result (red curve). The recovered signal has a fidelity of 98.48% in pulse shape while the pulse duration is 91.4 fs. Fig. S3(b) shows the compressive result of a 125 fs pulse. The fidelity is 97.88% while the pulse duration is 110.0 fs. The main limiting factor in optical pulse measurement is the instability induced by self-phase modulation. The instability not only leads to a worse SNR (less than 70 in delay stage data), but also results in an irregular but large intensity fluctuation at peak. We expect that this noise should vanish if one uses optical grating or other devices to introduce chirp. Therefore, a better recovery should be available for real optical pulses whose pulse duration are not extended by nonlinear effects. To get a more accurate CS recovery, one can also intentionally chirp, for example using time lenses, the optical pulses to a longer level and then use our CTSPI to measure it<sup>10–12</sup>.

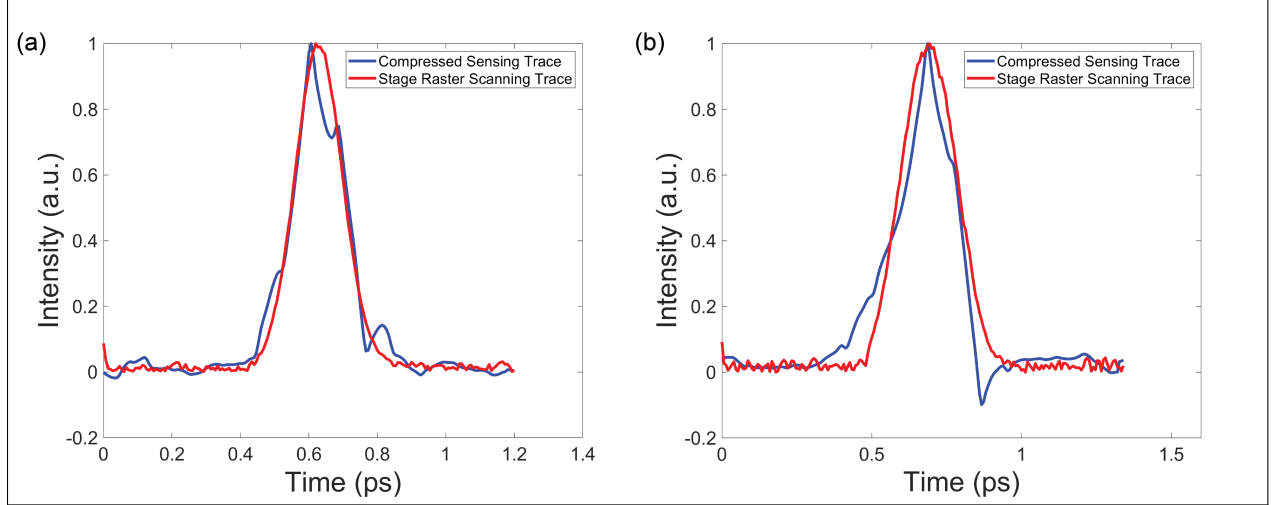

FIG. S3: (a): 90 fs pulse duration. (b): 125 fs pulse duration. Both CS results are measured at 80% CR to include enough high frequency components. The delay stage data has a temporal resolution of 6.67 fs. Both data have averaging.

#### IV. MEASURE THE TEMPORAL INTERVAL OF PULSE TRAIN

As what we show in the main paper, the theoretical temporal interval, which is the temporal resolution in our CTSPI system, can be calculated as:  $\Delta\tau = \sin(2\alpha)d/c$ . Therefore, we can find a theoretical value of 14.66 fs. To experimentally measure the temporal interval  $\Delta\tau$ , we first prepare a pulse train which is the same as what show in the middle figure of Fig. 1(c). Each effective TFO replica consists of 5 DMD columns, which means 5 columns are set to 'on' state. There are 15 DMD columns are set to 'off' state between two effective replicas, and each DMD column corresponds to one temporal interval  $\Delta\tau$ . Therefore, the separation between the peaks of two adjacent effective TFO replicas is 20 DMD columns, which is  $20\Delta\tau$  in the time domain. Since there are 30 effective replicas at the 'on' state, the separation between the first effective replica to the last effective replica is 580 DMD columns, which is  $580\Delta\tau$ . We then calculate the temporal separation  $\Delta T$  by measuring the position of the first effective replica and the last effective replica in 9 measurements. The temporal interval can be found as:  $\Delta\tau = \Delta T/580 = 16.00$  fs with a standard deviation of 0.01 fs. Note that 0.01 fs is the average uncertainty of each micromirror, and the uncertainty of the entire pulse train is 6.08 fs, which corresponds to an uncertainty of  $1.82 \mu\text{m}$  in spatial separation between the first and last effective replica. The  $1.82 \mu\text{m}$  spatial uncertainty is

a reasonable number according to the performance of our translation stage. Therefore, we believe that the temporal resolution induced by each micromirror is  $16.00 \pm 0.01$  fs.

## V. SIMULATION

A Matlab code is developed to simulate our TFO gate and CTSPI based on the theoretical model in Supplementary Information Section I. We first simulate the results shown in Fig. 2 in the main manuscript. As shown in Fig. S4, our experimental data precisely matches our simulation results. When the CR is 20%, both experimental and simulation data show the lack of high frequency components above 1.5 THz. Meanwhile, as what we discuss in the main manuscript, the weak side lobe at 2.4 THz, which corresponds to the sampling frequency of the 25 th row of the Walsh-ordered Hadamard Matrix (WOHM), is also verified by simulation. When the CR goes to 30%, the main part of the spectrum has been accurately recovered except for the weak side lobe, which is also observed in our experimental data. When the CR goes to 40%, the side lobe disappears and the spectrum of the CS recovered pulse is almost identical to original spectrum. Therefore, these simulation results indicate that our experimental data has a high agreement with the theoretical model.

We then focus on the role of pulse duration of the input pulse in TFO, which has a critical impact to TFO outputs. Basically, all TFO replicas are coherent unless the input pulse is spatially incoherent. Therefore, due to the long pulse duration, the interference between adjacent two or more sub-pulses will result in temporal structures under control. For example, in Fig. S2(a), when the input pulse has a duration of 80 fs and all columns are on, we can get a 9.73 ps long pulse in the time domain. As shown in Fig. S5(a)-(c), even when we separate two effective TFO copies, each one is the coherence interference of 4 TFO copies, with 192 fs, one still cannot get a unit contrast of pulse trains when the pulse duration is longer than 60 fs. If we further reduce the separation to 64 fs, we can only get pulse trains with unit contrast when the input pulse duration is around 16 fs. When no separation is added between two effective TFO copies, a 8.19 ps long top-hat pulse is generated in the time domain even the input pulse duration is 40 fs. Pulse trains with a unit contrast are only available with input pulse duration is equal to 10 fs if there is no additional separation between adjacent replicas.

Then we turn to figure out the impact of pulse duration on recovered THz signals. In fact,

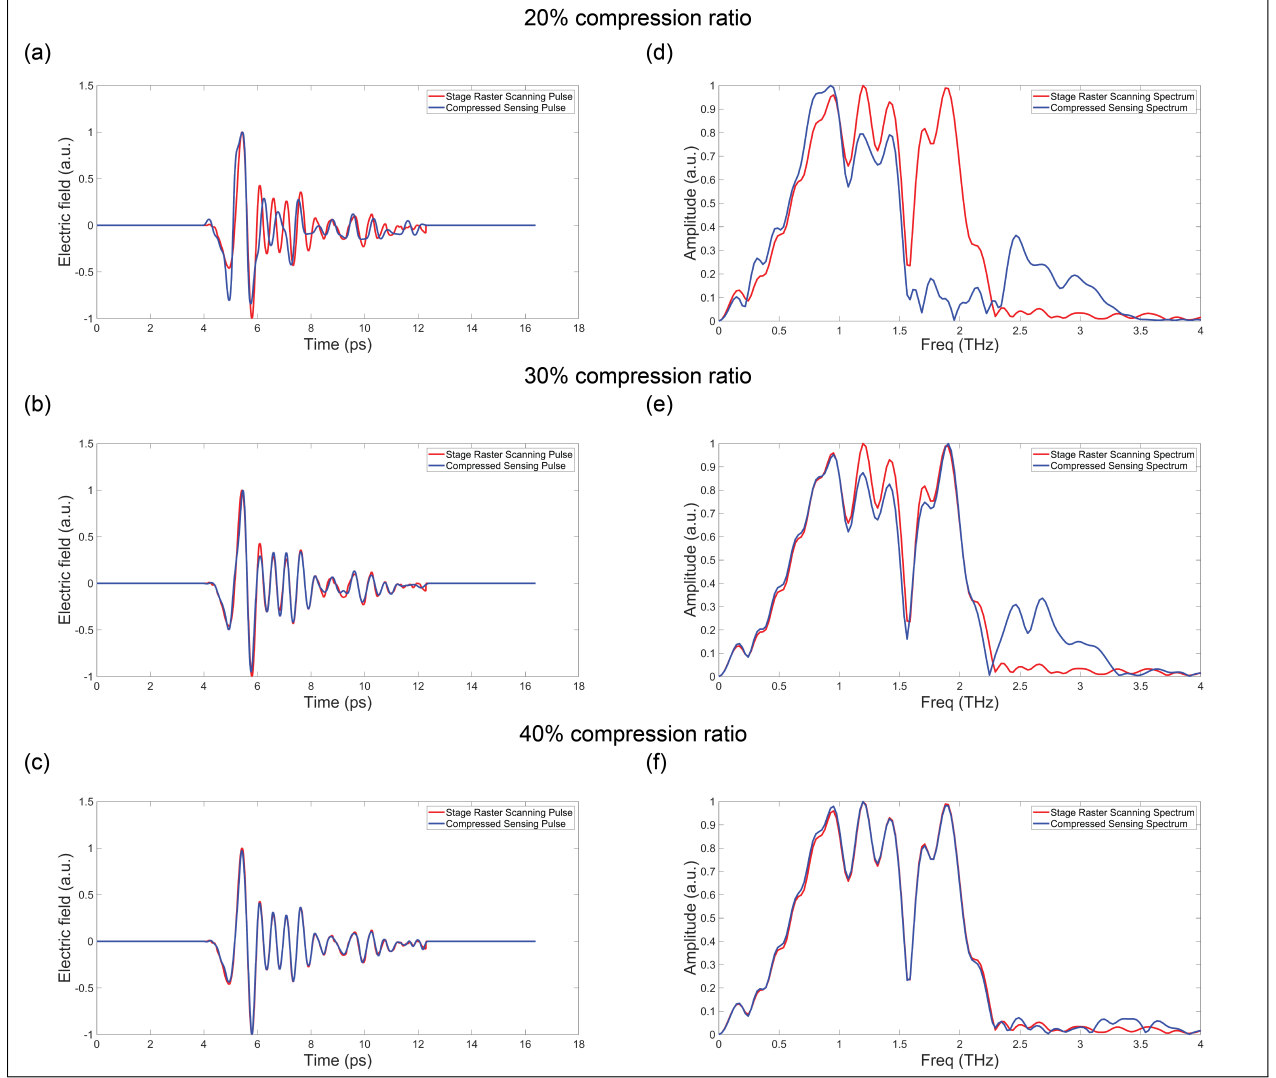

FIG. S4: (a)-(c): Recovered THz pulses at different CRs: 20%, 30% and 40% respectively. (d)-(f): Corresponding spectra at different CRs: 20%, 30% and 40% respectively.

we find that pulse duration, which leads to imperfections in pulse trains, only significantly affect the quality of pulses recovered by WOHM directly. Pulses recovered by CS, even both methods use the same encoding method, have similar fidelity and RMSE (difference less than 0.5%) under different pulse durations. As shown in Fig. S6(a)-(c), when input pulse duration is long and pulse trains have poor contrasts, THz signals recovered by WOHM have both over-estimations and under-estimations compared to original signals. This effect will get weaker when the pulse duration becomes short and the contrast of pulse trains gets close to unit. However, when pulse duration becomes ultra-short, for example 16 fs, one would expect the pixelization effect in the recovered THz signal as shown in Fig. S6(g) and

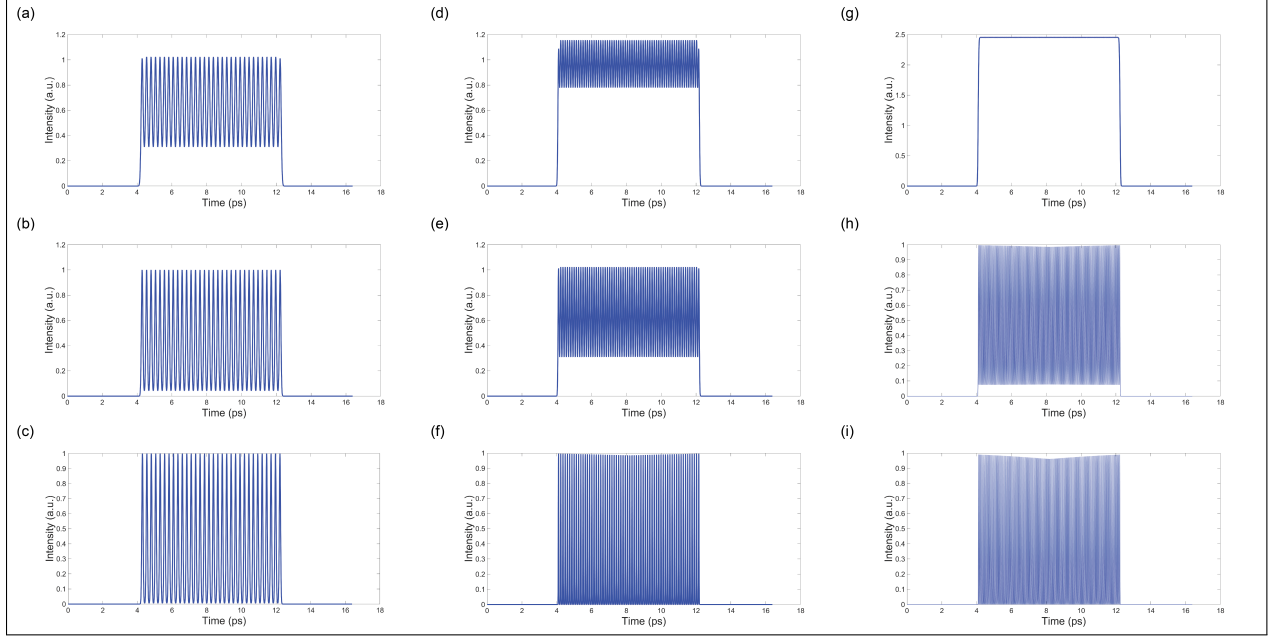

FIG. S5: (a)-(c): Pulse trains with different input pulse duration: 100 fs, 80 fs and 60 fs respectively. The temporal separation between two effective columns is equal to 192 fs. The contrast in (a) is 53.59% while it becomes 91.97% in (b), which matches our experimental observation. (d)-(f): Pulse trains with different input pulse duration: 60 fs, 40 fs and 16 fs respectively. The temporal separation between two effective columns is equal to 64 fs. The contrast in (d) is 19.43% which is too poor to use. The contrast becomes 53.52% in (e) which is good enough for both CTSPI and WOHM recovery. Pulse trains with different input pulse duration: 40 fs, 16 fs and 10 fs respectively. The temporal separation between two effective columns is equal to 16 fs. The contrast in (h) is 86.06%.

(h). As a comparison, THz signals recovered by CS, shown in Fig. S6(d)-(f) and (i), are much less affected by pulse duration and the quality of pulse trains, which demonstrates the robustness of our CTSPI. Therefore, our CTSPI is more robust against temporal fluctuations of the input pulse of TFO gate.

Next, we will demonstrate that our CTSPI is also robust against imperfections in TFO gate. We first prepare a simple distortion by making the envelop of pulse trains asymmetric. The ratio between the maximum and minimum in Fig. S7(a) is about 10, which is the same as the pulse train shown in Fig. 3(c). As one can see in Fig. S5(b), asymmetric pulse trains lead to the over-estimation at the tail of THz pulse and the under-estimation at the beginning of THz pulse when we use WOHM recovery directly. However, the defects from

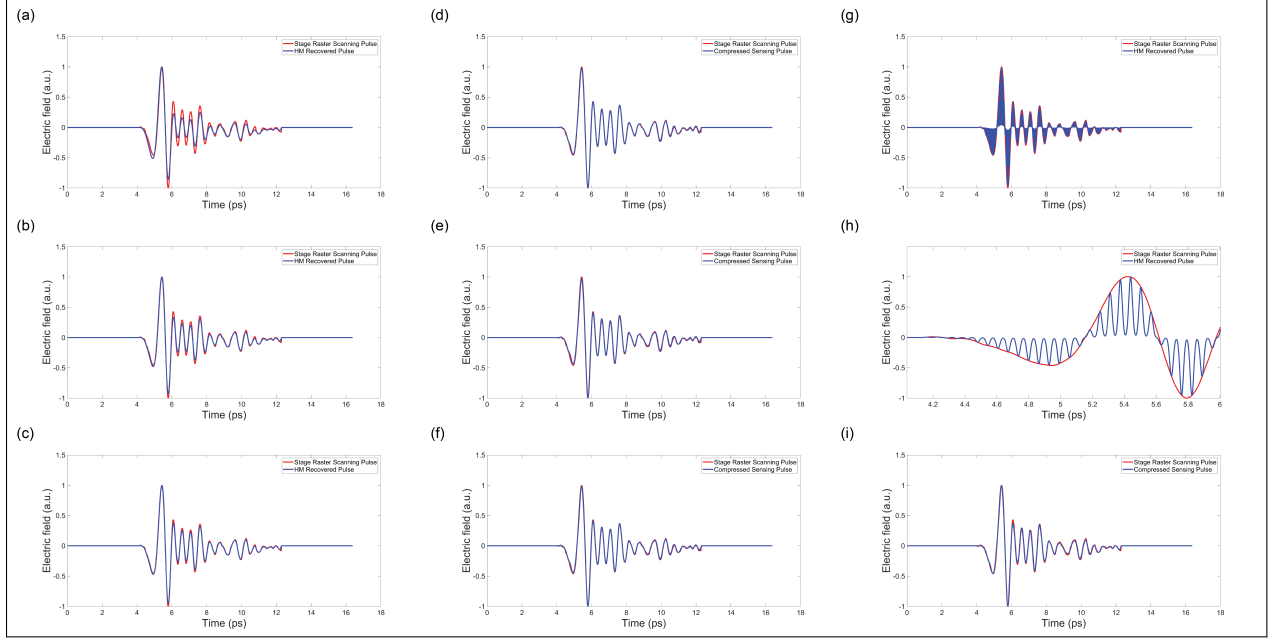

FIG. S6: (a)-(c): Recovered THz pulses using WOHM directly. The encoding process is the same as what we do in the experiment, i.e. each row of WOHM is represented by the sum of 4 sub-rows, which results in the corresponding pulse trains shown in Fig. S5(a)-(c) respectively. (d)-(f): Recovered THz pulses using CS and pulse trains in Fig. S5(a)-(c) respectively. CR is 40% for all three recoveries. (g): Recovery using WOHM directly. The pulse duration is 16 fs. (h): The zoom-in figure of 4-6 ps in (g). (i): CS recovery with a pulse duration of 16 fs.

the distorted TFO gate do not affect the performance of CTSPI (Fig. S7(c)). Then we make the distortion more complicated by moving the Fourier plane of DMD 25 mm away from the detection crystal. Due to the spread of k-vectors of different TFO replicas, each copy will intersect with different transverse position of the THz pulse. Considering the Gaussian distribution of the THz pulse and the asymmetric structure of pulse trains, the measured envelop of pulse trains at the detection crystal plane have an irregular envelop as shown in Fig. S7(d). The abnormal envelop of pulse trains leads to the over- and under-estimation of THz pulses. Nevertheless, our THz pulse recovered by CS is still robust to this more complicated distortion. The experimental verification and explanation of these two distortions have been shown in Fig. 3 of the main manuscript. In fact, the envelop of pulse trains plays a much less important role in CS recovery than WOHM or random recovery. One can even use a highly distorted TFO gate generating random intensity envelop of pulse

trains to recover THz signals using our CTSPI approach. The results are shown in Fig. S7(g)-(i). One can figure out that the random intensity envelop of pulse trains leads to a THz pulse with randomly distributed under- and over-estimations when WOHM recovery is used. However, in Fig. S7(i), the THz signal recovered by CS only gets slightly affected. Therefore, based on both experimental verification and theoretical analysis, we can claim that, as long as the correlation between temporal position of each TFO replica and intensity envelope of the entire pulse train is not destroyed, the recovered THz pulse will be robust against distortions on TFO gate.

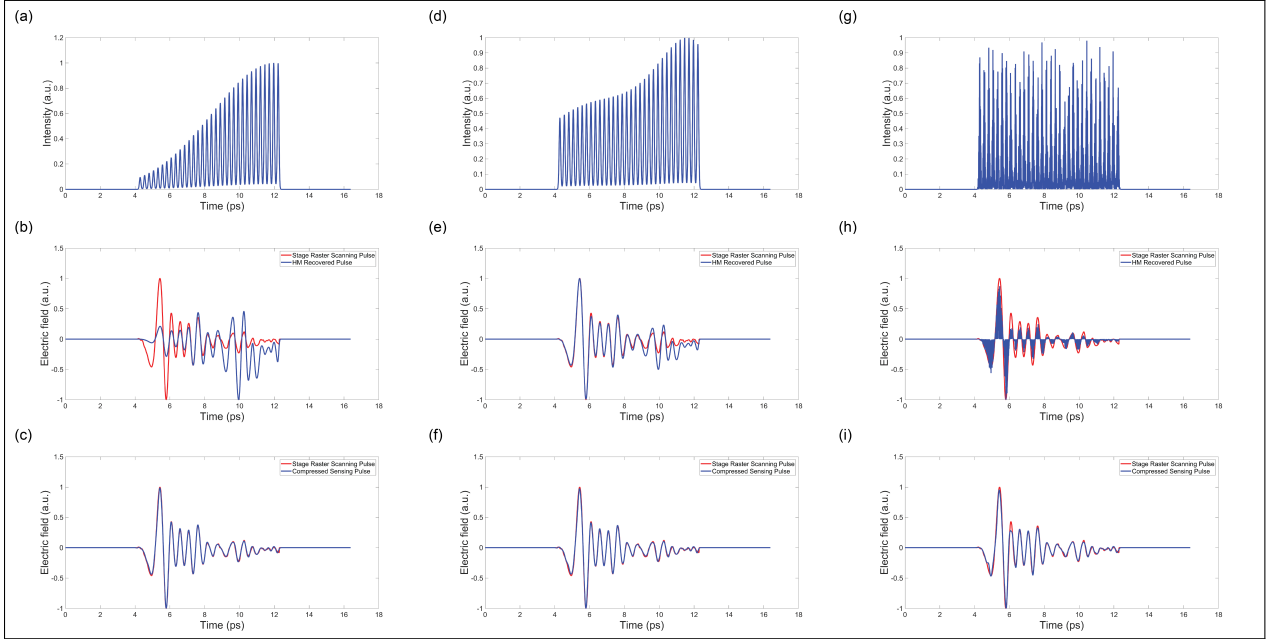

FIG. S7: (a)-(c): Recovered THz pulses using asymmetric pulse trains generated by the temporally distorted TFO gate. (d)-(f): Recovered THz pulses using asymmetric pulse trains located 25mm out of the detection crystal plane. (g)-(i): Recovery based on a random envelop of pulse trains. The CR is 40% for all CS recoveries.

## VI. MACHINE LEARNING

A simple 12-layer CNN is developed to classify the compressive signals of different samples under weak SNR, and the architecture is shown in Fig. S8. The input signal layer ( $1 \times 128$ ) is connected to the first convolution layer with 16  $1 \times 4$  filters. Then a batch normalization layer and a ReLu layer are implemented sequentially, which normalizes the activations and

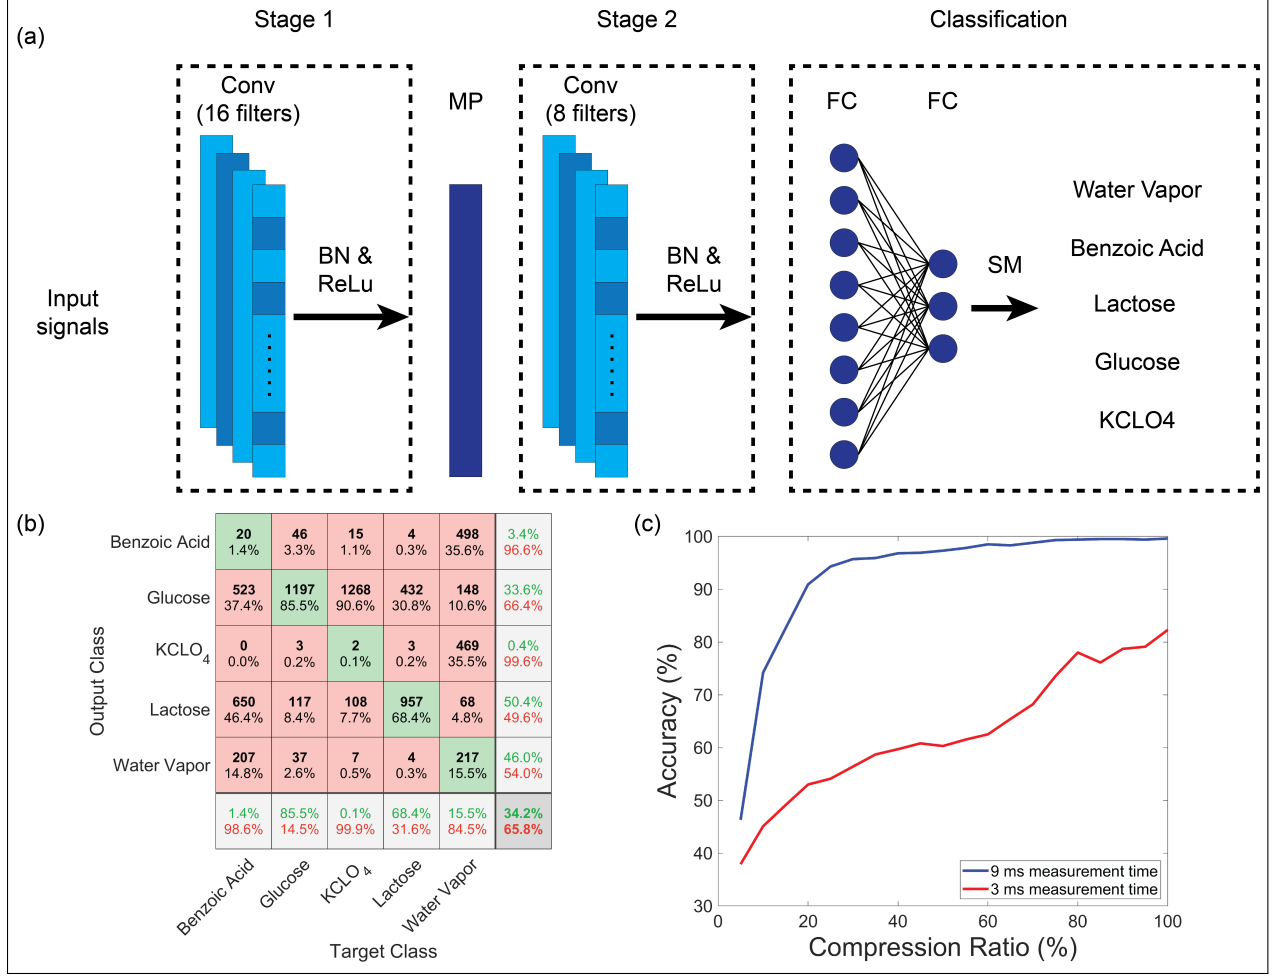

FIG. S8: (a): Architecture of our CNN. Conv stands for convolution layer while BN and ReLu stand for batch normalization layer and rectified linear unity layer respectively. MP is the maxpooling layer and FC is the fully connected layer. SM is the softmax layer. (b): Confusion matrix before training. Due to the poor SNR, the classification accuracy is only 34.2%. The green numbers are accuracy of each sample while the red numbers are failure probabilities. The CR is 40%. (c): The classification accuracy as a function of CR. Two groups of data are measured with 9 ms measurement time and 3 ms measurement time. Each data point in (c) is the average over 5 trained CNN.

is the nonlinear activation function respectively. After the first stage, a max pooling layer with a  $1 \times 2$  pooling size is used to localize the features. Then the second stage starts with another convolution layer consisting of 8  $1 \times 4$  filters. Similar to the first stage, a batch normalization and a ReLu layer are used. After this, we enter the classification stage with two fully connected layers (8 neurons and 3 neurons respectively). At last, a softmax layer,

which normalizes the output from the fully connected layer, and a classification layer are adopted.

Five samples are used to train this CNN. Each sample has 1000 sets of data from our ultrafast THz TDS system so that in total 5000 sets of data are used for training. Each set of data is measured under a sample rate of 20 Hz or 50 Hz with an integration time (time constant) of 3 ms, which corresponds to acquisition times for each DMD pattern of 50 ms and 20 ms respectively. However, due to the limited data readout time between lock-in amplifier and computer ( $\sim 15$  ms), there are only 3 data points inside each acquisition time of 50 ms. For the same reason, only 1 data point for the acquisition time equal to 20 ms. Therefore, the effective measurement time of each DMD pattern in ML is 9 ms (for 50 ms acquisition time) and 3 ms (for 20 ms acquisition time). Since our THz pulse is attenuated to 3 times weaker, the final SNR of these data sets is about 10 (for 20 Hz sampling rate) or 17 (for 50 Hz sampling rate) times weaker than the data shown in Fig. 2 and 3. Due to the poor SNR, the accuracy of the successful classification without training is less than 35%. For example, 34.20% in the confusion matrix shown in Fig. S8(b).

The training process shuffles these sets of data at the beginning of every epoch and 6 epochs are used. In order to provide a more stable network, a batch size of 150 sets of data is used, which further leads to the maximal number of iterations at 60. The entire training process takes about 400 s with a constant training rate of 0.01. We then use 2000 sets of data (400 sets of each sample) to validate the performance of our CNN, and the successful classification probability is about 97.5% at 40% CR. The relation between the classification accuracy and CR is shown in Fig. S8(c). When the sampling rate is 20 Hz (9 ms measurement time), the accuracy rises up soon when the CR goes from 5% to 20%, then starts to converge and increase slowly. This matches the fidelity data we show in Fig. S1 since both the classification accuracy and fidelity quantify the amount of information that we can get from the compressive signal. A larger CR always indicates that more information is included in the analysis. As a comparison, due to the poor SNR, the accuracy does not converge when the sampling rate is 50 Hz (3 ms measurement time). This indicates that a more complicated training with more data is required when SNR is poor.

## VII. PERFORMANCE COMPARISON TO OTHER TECHNIQUES USING DELAY STAGE, CAMERAS, SPECTROMETERS OR TIME LENS

The conventional way for measuring ultrafast signals is using mechanical stages to scan the time delay. The advantage of our method over a mechanical delay stage mainly comes from the use of CS algorithm and DMD, which provide a better SNR for weak signals, a faster sampling speed, a better sampling accuracy and a higher flexibility. The robustness against noise of our TFO enabled CTSPI can be found in Fig. S9. Both the CTSPI data and delay stage data are measured with KClO<sub>4</sub> sample. The SNR of the delay stage data without averaging is 9.67 while the SNR of the delay stage data averaging over 9 sets of data is 30.57. As one can see, even our recovered data has no averaging and a CR at 40%, it is a more accurate measurement of the THz signal than the delay stage data without averaging. Therefore, our CTSPI is not only fundamentally more efficient than conventional methods, but also more robust to noise from a practical point of view.

In theory, the measurement time of raster scanning using delay stage scales up with the measurement points  $N$  in the 1-D temporal measurement, and scales up with  $N^2$  in spatial characterization. Therefore, if one wants to fully characterize the THz pulse in both space and time domain, the measurement time will scale up with  $N^3$ , which leads to a huge time consumption. However, CS can fundamentally enhance the measurement efficiency by a factor more than 3 as what we shown in the main paper. That is to say, for a 3-D characterization problem, the time consumption will be only 1/27 of the raster scanning method using delay stage. Therefore, if we combine our previous CS method on THz spatial sampling with the current temporal CS approach, the measurement efficiency will be significantly improved<sup>7</sup>. From a practical point of view, as what we mention in the main paper, our system is faster than a delay stage (4 Hz)<sup>13</sup>, which is working at 10 Hz. However, we does not fully utilize the advantage of DMD in sampling speed, and there are two limiting factors stop us from fast measurements at kHz level, which is the potential speed limit of the system. The first limiting factor is the poor SNR of our THz pulse. The signal becomes noisy when the integration time (time constant) on lock-in amplifier is below 10 ms and hence the recovered pulse has a poor quality (as shown in Fig. 4 in the paper). The second limiting factor is the communication speed between lock-in amplifier and our data acquisition program. The data read-out time from lock-in amplifier to our

computer program is about 15 ms. Therefore, the maximal sampling rate with this lock-in amplifier is about 66.67 Hz, which is far below the speed limit of DMD. Hence, to improve the measurement speed to kHz level, not only a stronger THz pulse is required, a faster digital signal processing card with synchronization is also necessary. Luckily, both requirements are not hard to accomplish if the hardware are upgraded. For example, researchers have demonstrated the possibility of using a commercially available fiber-based THz system to generate high SNR THz signals, and perform fast measurement over 2 kHz with a fast data acquisition card<sup>14</sup>. Even though due to the long response time of silicon, the speed of their scheme cannot go beyond 4 kHz, our methods, including our previous spatial CS approach, have no such limitation<sup>7</sup>. Therefore, we believe that, after upgrading the hardware, kHz-level sampling rate is applicable to our approach, and it is even possible to reach the speed limit of DMD at 20 kHz.

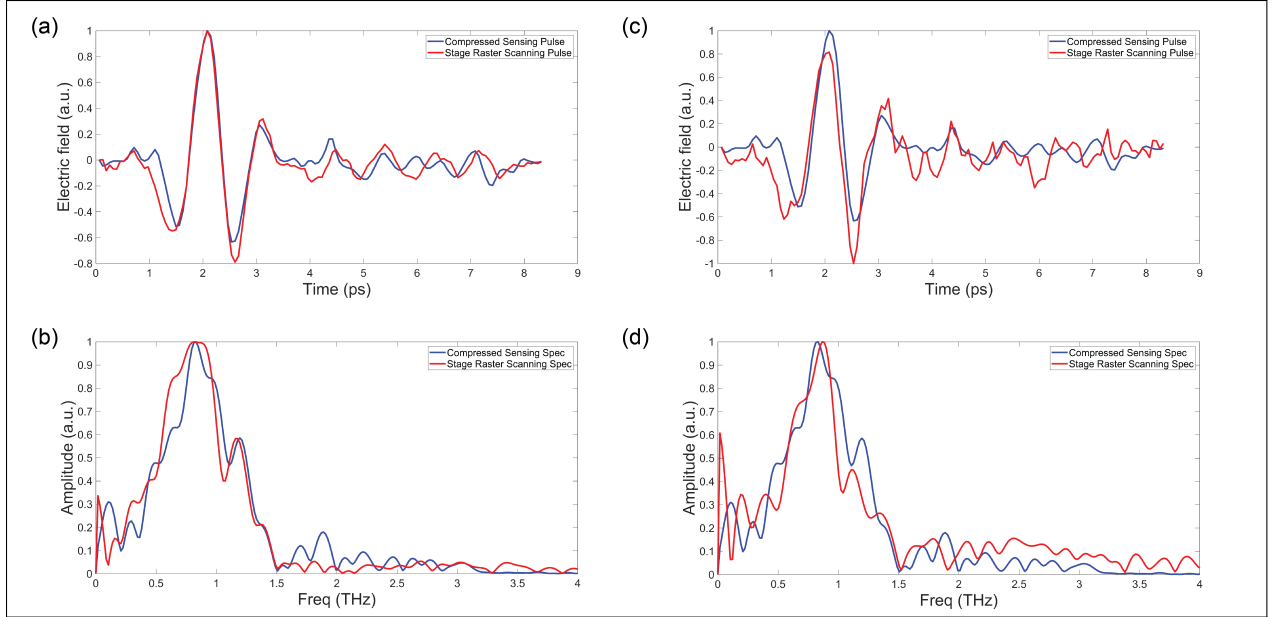

FIG. S9: (a)-(b): Recovered THz field and spectrum compared to THz field measured by delay stage averaging over 9 measurements. (c)-(d): Recovered THz field and spectrum compared to THz field measured by delay stage without averaging. The fidelity in (a) is 94.20% and the RMSE is 9.51%. As a comparison, the fidelity in (c) is 80.80% and the RMSE is 17.56%. Note that, the fidelity between two delay stage data is 87.88% and the RMSE is 10.65%. The integration time of lock-in amplifier for all data shown in this figure is 30 ms.

Comparing to methods using cameras or spectrometers, our approach is applicable to both weak and strong pulses. Even though cameras and spectrometers enable the possibility of single-shot measurements, they cannot effectively measure weak pulses. For example, these methods usually require the use of  $\mu\text{J}$ -to- $\text{mJ}$ -level pump pulse to generate  $\text{nJ}$ -to- $\text{pJ}$ -level THz pulses<sup>15–21</sup>. As a comparison, our approach only needs  $\text{nJ}$ -level pump pulses, and is capable of measuring  $\text{fJ}$ -level THz pulses. Hence, the sensitivity of our system is at least 3 orders of magnitude better than the camera- or spectrometer-based methods. Furthermore, when pulses become weak, these single-shot measurement methods will need to average over multiple shots to provide a good SNR, which will result in a slow measurement speed.

Temporal imaging based on time lenses is another way to measure ultrafast signals. The basic idea is to stretch the pulse using time lenses to a longer level so that fast photodiodes are able to measure the optical pulses<sup>10–12</sup>. However, one has to design and fabricate complicated time lenses, which usually lacks flexibility to diverse application scenarios. In the sensing process, fast photodiodes is required as well, and one cannot beat Nyquist sampling limit with this approach. Therefore, our approach has a better flexibility, and is fundamentally more efficient and convenient.

## REFERENCES

- <sup>1</sup>Wu, Q. & Zhang, X.-C. Free-space electro-optic sampling of terahertz beams. *Applied Physics Letters* **67**, 3523–3525 (1995).
- <sup>2</sup>Lee, Y.-S. *Principles of terahertz science and technology*, vol. 170 (Springer Science & Business Media, Berlin, 2009).
- <sup>3</sup>Zhang, X.-C. & Xu, J. *Introduction to THz wave photonics*, vol. 29 (Springer, New York City, 2010).
- <sup>4</sup>Candès, E. J. & Wakin, M. B. An introduction to compressive sampling. *IEEE Signal Processing Magazine* **25**, 21–30 (2008).
- <sup>5</sup>Romberg, J. Imaging via compressive sampling. *IEEE Signal Processing Magazine* **25**, 14–20 (2008).
- <sup>6</sup>Candès, E. & Romberg, J. Sparsity and incoherence in compressive sampling. *Inverse Problems* **23**, 969 (2007).
- <sup>7</sup>Zhao, J., Yiwen, E., Williams, K., Zhang, X.-C. & Boyd, R. W. Spatial sampling of

- terahertz fields with sub-wavelength accuracy via probe-beam encoding. *Light: Science & Applications* **8**, 1–8 (2019).
- <sup>8</sup>Ryczkowski, P., Barbier, M., Friberg, A. T., Dudley, J. M. & Genty, G. Ghost imaging in the time domain. *Nature Photonics* **10**, 167–170 (2016).
- <sup>9</sup>Li, C. Compressive sensing for 3d data processing tasks: applications, models and algorithms. Tech. Rep. (2011).
- <sup>10</sup>Kolner, B. H. & Nazarathy, M. Temporal imaging with a time lens. *Optics Letters* **14**, 630–632 (1989).
- <sup>11</sup>Salem, R. *et al.* Optical time lens based on four-wave mixing on a silicon chip. *Optics Letters* **33**, 1047–1049 (2008).
- <sup>12</sup>Foster, M. A. *et al.* Ultrafast waveform compression using a time-domain telescope. *Nature Photonics* **3**, 581–585 (2009).
- <sup>13</sup>Newport Precision Long-Travel & High-Speed Motorized Actuators. [https://www.newport.com/mam/celum/celum\\_assets/resources/LTA\\_-\\_User\\_s\\_Manual.pdf?1](https://www.newport.com/mam/celum/celum_assets/resources/LTA_-_User_s_Manual.pdf?1) (2018).
- <sup>14</sup>Stantchev, R. I., Yu, X., Blu, T. & Pickwell-MacPherson, E. Real-time terahertz imaging with a single-pixel detector. *Nature Communications* **11**, 1–8 (2020).
- <sup>15</sup>Jiang, Z. & Zhang, X.-C. Single-shot spatiotemporal terahertz field imaging. *Optics Letters* **23**, 1114–1116 (1998).
- <sup>16</sup>Shan, J. *et al.* Single-shot measurement of terahertz electromagnetic pulses by use of electro-optic sampling. *Optics Letters* **25**, 426–428 (2000).
- <sup>17</sup>Kim, K. *et al.* Single-shot, interferometric, high-resolution, terahertz field diagnostic. *Applied Physics Letters* **88**, 041123 (2006).
- <sup>18</sup>Kim, K., Yellampalle, B., Taylor, A., Rodriguez, G. & Glowacki, J. Single-shot terahertz pulse characterization via two-dimensional electro-optic imaging with dual echelons. *Optics Letters* **32**, 1968–1970 (2007).
- <sup>19</sup>Kawada, Y., Yasuda, T., Nakanishi, A., Akiyama, K. & Takahashi, H. Single-shot terahertz spectroscopy using pulse-front tilting of an ultra-short probe pulse. *Optics Express* **19**, 11228–11235 (2011).
- <sup>20</sup>Teo, S. M., Ofori-Okai, B. K., Werley, C. A. & Nelson, K. A. Invited article: Single-shot thz detection techniques optimized for multidimensional thz spectroscopy. *Review of Scientific Instruments* **86**, 051301 (2015).

<sup>21</sup>Zheng, S. *et al.* Common-path spectral interferometry for single-shot terahertz electro-optics detection. *Optics Letters* **42**, 4263–4266 (2017).
